# Supplementary material for: 3DGS-Avatar: Animatable Avatars via Deformable 3D Gaussian Splatting
Source: arXiv:2312.09228 source file (2024-04-04)
Supplement: Supplementary file 1 [file quantitative.tex]

\section{Additional Quantitative Results}
\label{sec:supp_quantitative}

\subsection{Comparison to Instant-NVR}
In the main paper we claim that the metrics from Instant-NVR are not directly comparable to other baselines as they use refined ZJU-MoCap which updates the foreground masks, the SMPL fittings and the camera parameters. Hence we train our model on the refined dataset for a fair quantitative comparison, reported in \cref{tab:supp_nvr}. Though Instant-NVR provides high PSNR metric, they produce images with poor visual quality and little details as shown in 
% Fig.~\textcolor{red}{3}
\cref{fig:zju_qualitative}
of the main paper and \cref{fig:supp_quality_zju_nv}, since PSNR is widely known to be in favor of smooth results. It is clearly shown that our method significantly outperforms Instant-NVR in LPIPS, which is the most informative criterion on monocular setup.

\begin{table*}
\setlength{\fboxsep}{0pt}
% \scriptsize
% \fontsize{6}{7}\selectfont
 \caption{\textbf{Comparison to Instant-NVR on refined ZJU-MoCap~\cite{instant_nvr}.}
 }
 \label{tab:supp_nvr}
 \centering
 \begin{tabular}{ l|ccc|ccc|ccc}
 \toprule
 Subject:                                      
 & \multicolumn{3}{c}{377}                                                 
 & \multicolumn{3}{c}{386}                                                 
 & \multicolumn{3}{c}{387}
 \\ %\hline
Metric:             
& PSNR$\uparrow$
& SSIM$\uparrow$
& LPIPS$\downarrow$    
& PSNR$\uparrow$
& SSIM$\uparrow$
& LPIPS$\downarrow$    
& PSNR$\uparrow$
& SSIM$\uparrow$
& LPIPS$\downarrow$
 \\\hline
 Instant-NVR*~\cite{instant_nvr}
 & \textbf{31.28} 
 & \textbf{0.9789 }
 & 25.37
 & 33.71 
 & 0.9770 
 & 32.81
 & 28.39 
 & 0.9640 
 & 45.97
 \\
 Ours*                                 
 & 30.96
 & 0.9778
 & \textbf{19.85}
 & \textbf{33.94}
 & \textbf{0.9784}
 & \textbf{24.70}
 & \textbf{28.40}
 & \textbf{0.9656}
 & \textbf{32.96}
 \\ 
 \bottomrule
 \end{tabular}
 \begin{tabular}{ l|ccc|ccc|ccc}
 \toprule
 Subject:                   
 & \multicolumn{3}{c}{392}                   
 & \multicolumn{3}{c}{393}                    
 & \multicolumn{3}{c}{394}
 \\ %\hline
Metric:        
& PSNR$\uparrow$
& SSIM$\uparrow$
& LPIPS$\downarrow$   
& PSNR$\uparrow$
& SSIM$\uparrow$
& LPIPS$\downarrow$    
& PSNR$\uparrow$
& SSIM$\uparrow$
& LPIPS$\downarrow$
 \\\hline
 Instant-NVR*~\cite{instant_nvr}
 & 31.85 
 & 0.9730 
 & 39.47
 & \textbf{29.56 }
 & 0.9641 
 & 46.16
 & \textbf{31.32 }
 & \textbf{0.9680 }
 & 40.63 
 \\
 Ours*          
 & \textbf{32.10}
 & \textbf{0.9739}
 & \textbf{29.20}
 & 29.30
 & \textbf{0.9645}
 & \textbf{34.03}
 & 30.74
 & 0.9662
 & \textbf{31.00}
 \\ 
 \bottomrule
 \end{tabular}
\end{table*}

\subsection{Comparison to MonoHuman}

We train MonoHuman models on the same data split and report the quantitative results in \cref{tab:supp_monohuman}. Our method outperforms MonoHuman on all subjects.

\begin{table*}
\setlength{\fboxsep}{0pt}
\scriptsize
\fontsize{9}{10}\selectfont
 \caption{\textbf{Comparison to MonoHuman on ZJU-MoCap.}
 }
 \label{tab:supp_monohuman}
 \centering
 \begin{tabular}{ lcc|ccc|ccc|ccc}
 \toprule
 Subject:                       
 & \multicolumn{2}{c}{}
 & \multicolumn{3}{c}{377}                                                 
 & \multicolumn{3}{c}{386}                                                 
 & \multicolumn{3}{c}{387}
 \\ %\hline
Metric:             
& GPU$\downarrow$
& FPS$\uparrow$
& PSNR$\uparrow$
& SSIM$\uparrow$
& LPIPS$\downarrow$    
& PSNR$\uparrow$
& SSIM$\uparrow$
& LPIPS$\downarrow$    
& PSNR$\uparrow$
& SSIM$\uparrow$
& LPIPS$\downarrow$
 \\\hline
 MonoHuman~\cite{yu2023monohuman}
 & 100h
 & 0.1
 & 29.12
 & 0.9727
 & 26.58
 & 32.94
 & 0.9695
 & 36.04
 & 27.93
 & 0.9601
 & 41.76
 \\
 Ours         
 & \textbf{0.5h}
 & \textbf{50}
 & \textbf{30.64}
 & \textbf{0.9774}
 & \textbf{20.88}
 & \textbf{33.63}
 & \textbf{0.9773}
 & \textbf{25.77}
 & \textbf{28.33}
 & \textbf{0.9642}
 & \textbf{34.24}
 \\ 
 \bottomrule
 \end{tabular}
 \begin{tabular}{ lcc|ccc|ccc|ccc}
 \toprule
 Subject:   
 & \multicolumn{2}{c}{}
 & \multicolumn{3}{c}{392}                   
 & \multicolumn{3}{c}{393}                    
 & \multicolumn{3}{c}{394}
 \\ %\hline
Metric:        
& GPU$\downarrow$
& FPS$\uparrow$
& PSNR$\uparrow$
& SSIM$\uparrow$
& LPIPS$\downarrow$   
& PSNR$\uparrow$
& SSIM$\uparrow$
& LPIPS$\downarrow$    
& PSNR$\uparrow$
& SSIM$\uparrow$
& LPIPS$\downarrow$
 \\\hline
 MonoHuman~\cite{yu2023monohuman}
 & 100h
 & 0.1
 & 29.50
 & 0.9635
 & 39.45
 & 27.64
 & 0.9566
 & 43.17
 & 29.15
 & 0.9595
 & 38.08
 \\
 Ours
 & \textbf{0.5h}
 & \textbf{50}
 & \textbf{31.66}
 & \textbf{0.9730}
 & \textbf{30.14}
 & \textbf{28.88}
 & \textbf{0.9635}
 & \textbf{35.26}
 & \textbf{30.54}
 & \textbf{0.9661}
 & \textbf{31.21}
 \\ 
 \bottomrule
 \end{tabular}
\end{table*}
