# Supplementary material for: 3DGS-Avatar: Animatable Avatars via Deformable 3D Gaussian Splatting
Source: arXiv:2312.09228 source file (2024-04-04)
Supplement: Supplementary file 2 [file errata.tex]

\section{Errata}
\label{sec:supp_errata}

We first modify two minor errors in the main paper. In Tab.~\textcolor{red}{1},
% \cref{tab:comparison}
NeuralBody~\cite{peng2020neural} is able to be trained from monocular inputs despite its relatively poor performance. In Tab.~\textcolor{red}{3},
% \cref{tab:compare_peoplesnapshot}
we train our model for $30k$ iterations on PeopleSnapshot, which takes less than $45$ minutes instead of $30$ minutes. This, however, does not change the statement that our method achieves fast training.
